# Supplementary material for: Enhancing entropy and enthalpy fluctuations to drive crystallization in atomistic simulations
Source: arXiv:1612.03235 ancillary file (2017-03-28)
Supplement: Supplementary file 1 [file supplementalMaterial.pdf]

# Supplemental material to: Enhancing entropy and enthalpy fluctuations to drive crystallization in atomistic simulations

Pablo M. Piaggi, Omar Valsson, and Michele Parrinello

March 26, 2017

## 1 Collective variables

As described in the manuscript, we have employed two collective variables (CVs). The enthalpic CV is defined as,

$$s_H = \frac{U(\mathbf{R}) + PV}{N}, \tag{1}$$

where $U(\mathbf{R})$ is the potential energy, $P$ is the pressure, $V$ is the volume, and $N$ the number of atoms in the system[1]. The input for this CV in PLUMED 2[2] is:

```
ENERGY LABEL=ene

VOLUME LABEL=vol

COMBINE ...
 ARG=ene,vol
 POWERS=1,1
 COEFFICIENTS=1.,0.060221409
 PERIODIC=NO
 LABEL=enthalpy
... COMBINE

COMBINE ...
 ARG=enthalpy
 POWERS=1
 COEFFICIENTS=0.004
 PERIODIC=NO
 LABEL=enthalpyPerAtom
... COMBINE
```

where 0.060221409 kJ $mol^{-1}$ $nm^{-3}$ = 1 bar, and 0.004 is $1/N$ where $N = 250$ is the number of particles.

The entropic CV is based on the pair entropy (equation 1 of the manuscript) and defined as:

$$s_S = -2\pi\rho \sum_{k=1}^{n} \left[ g_m(r_k) \ln g_m(r_k) - g_m(r_k) + 1 \right] r_k^2 w_k \Delta r, \tag{2}$$

where $r_k = \frac{k-1}{n-1} r_{\max}$, $n$ is an integer that defines the number of steps in the integration, $r_{\max}$ is a cut off distance for the integration, $\Delta r = r_k - r_{k-1}$, $\mathbf{w} = (1/2, 1, 1, ..., 1, 1, 1/2)$ are the weights of the trapezoidal rule, $\rho$ is the density, and

$$g_m(r) = \frac{1}{4\pi N \rho r^2} \sum_{i \neq j} \frac{1}{\sqrt{2\pi\sigma^2}} e^{-(r-r_{ij})^2/(2\sigma^2)} \tag{3}$$

is a mollified radial distribution function with $N$ the number of atoms in the system, $r_{ij}$ is the distance between particles $i$ and $j$, and $\sigma$ a broadening parameter. For this work we have chosen $\Delta r = \sigma = 0.0125$ nm both for Na and Al. $r_{\max}$ was 0.65 nm and 0.7 nm for Na and Al, respectively. A PLUMED 2 input for this variable is:

```
PENTROPY ...
 LABEL=s2
 GROUPA=1-250
 NLIST
 MAXR=0.65
 SIGMA=0.0125
 NHIST=53
 NL_CUTOFF=0.7
 NL_STRIDE=10
... PENTROPY
```

where MAXR is $r_{\max}$, SIGMA is $\sigma$, NHIST is $n$, and the other keywords are standard in PLUMED 2 (see for instance COORDINATION). The source code for this CV will be made publicly available in the future.

We now give some useful definitions. The marginal probability distribution with respect to $s_H$ and $s_S$ is,

$$P(s_H, s_S) = \int d\mathbf{R} P(\mathbf{R}) \delta(s_H - s_H(\mathbf{R})) \delta(s_S - s_S(\mathbf{R})), \tag{4}$$

where $P(\mathbf{R})$ is the probability of observing configuration $\mathbf{R}$ in the simulated ensemble. In our case this is given by the isothermal-isobaric ensemble. It is possible to associate a free energy,

$$F(s_H, s_S) = -\frac{1}{\beta} \log P(s_H, s_S), \tag{5}$$

to the probability $P(s_H, s_S)$. $F(s_H, s_S)$ is generally referred to as free energy surface (FES).

Table 1: Simulations of Na performed with well tempered metadynamics. Summary of the parameters that were used: target temperature of the thermostat ($T$), biased CVs (CVs), bias factor of the well tempered distribution ($\gamma$), height of the gaussians ($w$), deviation of the gaussians in $s_H$ ($\sigma_{s_H}$), deviation of the gaussians in $s_S$ ($\sigma_{s_S}$), number of walkers, and total simulation time ($t$). In the first entry of the table we show all different temperatures for which the same parameters have been used.

| $T$ (K) | CVs | $\gamma$ | $w$ (kJ/mol) | $\sigma_{s_H}$ (kJ/mol) | $\sigma_{s_S}$ (k$_B$) | # walkers | $t$ (ns) |
|---|---|---|---|---|---|---|---|
| 300, 325, 350, 375, 400 | $s_H, s_S$ | 30 | 2.5 | 0.2 | 0.1 | 1 | 600 |
| 350 | $s_H$ | 30 | 2.5 | 0.2 | - | 1 | 600 |
| 350 | $s_S$ | 30 | 2.5 | - | 0.1 | 1 | 600 |

# 2 Sodium

We simulated Na using the embedded atom model (EAM) reported in ref. 3. Three EAM potentials for Na were developed in that article and we have employed the one they name Na1. This model has a melting temperature of 366 K according to their calculation and bcc is the minimum potential energy structure. The cohesive energy of the bcc lattice is $E_{\text{coh}}$ = 1.11 eV/atom = 107.1 kJ/mol/atom, and will be used to normalize the enthalpic CV in some of the figures.

## 2.1 Calculation of the Gibbs free energy surface

We calculated the FES $F(s_H, s_S)$ for Na at different temperatures. We have used well tempered metadynamics (WTMetaD)[4,5] and the variationally enhanced sampling (VES) method[6] in its well tempered variant[7].

**Well tempered metadynamics**

We first discuss the WTMetaD simulations. Details of the simulations that were carried out are shown in Table 1. At each temperature the final bias potential $V(s_H, s_S)$ was calculated through the summation of the gaussians deposited during the simulation. Then the FES $F(s_H, s_S)$ was calculated using the relation (up to an arbitrary constant),

$$F(s_H, s_S) = -\left(\frac{\gamma}{\gamma - 1}\right) V(s_H, s_S), \tag{6}$$

where $\gamma$ is the bias factor. Finally $P(s_H, s_S)$ was calculated from the FES using equation (5). In Figure SI-1 we show $P(s_H, s_S)$ for the 5 temperatures studied. From this plot

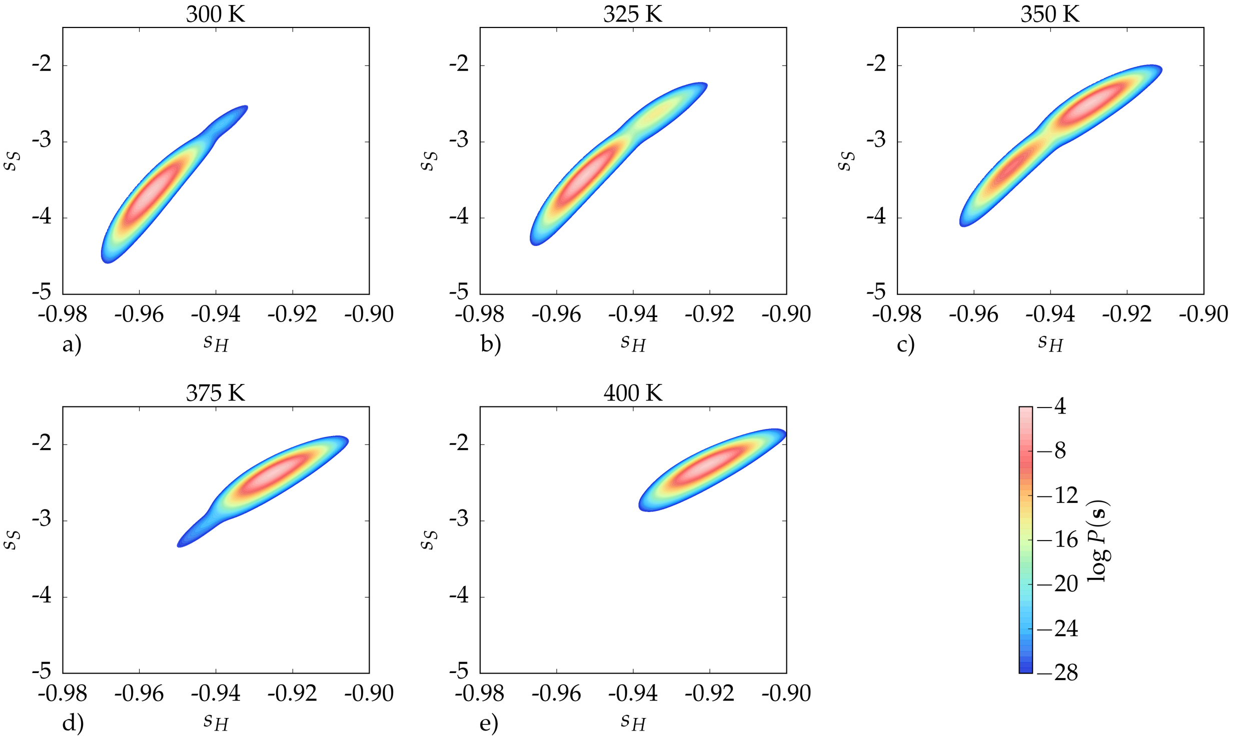


Figure SI-1: a)-e) Marginal probability distribution with respect to $s_H$ and $s_S$ for temperatures in the range 300-400 K for Na. $s_H$ is expressed in units of the cohesive energy and $s_S$ is in $k_B$.

one can observe that there are only one or two regions of high probability at each temperature. The region of high probability at high $s_H$ and $s_S$ corresponds to the liquid state, whereas the region of high probability at low $s_H$ and $s_S$ corresponds to a solid state. As the temperature is increased the liquid region grows at the expense of the solid one. At around 350 K the two states have a similar probability. At all temperatures the solid region contains only bcc configurations. It can also be seen that at around 300 K and 375 K the system is beyond the limits of metastability, and therefore only one minimum exists.

The difference in free energy between the liquid and solid basins $\Delta G_{S\to L}$ was calculated as:

$$\Delta G_{S\to L} = -\frac{1}{\beta}\log\left(\frac{\int_{\mathrm{L}} d\mathbf{s}e^{-\beta G(\mathbf{s})}}{\int_{\mathrm{S}} d\mathbf{s}e^{-\beta G(\mathbf{s})}}\right) \tag{7}$$

where $\mathbf{s}$ is the set of CVs $s_H$ and $s_S$, $G(\mathbf{s})$ is the FES calculated with equation (6) at a given simulation time, and the integrals are restricted to the liquid (L) and solid (S) basins, respectively. $\Delta G_{S\to L}$ as a function of simulation time is shown in Figure SI-2 a) for all the temperatures studied. The mean value and deviation of $\Delta G_{S\to L}$ are plotted

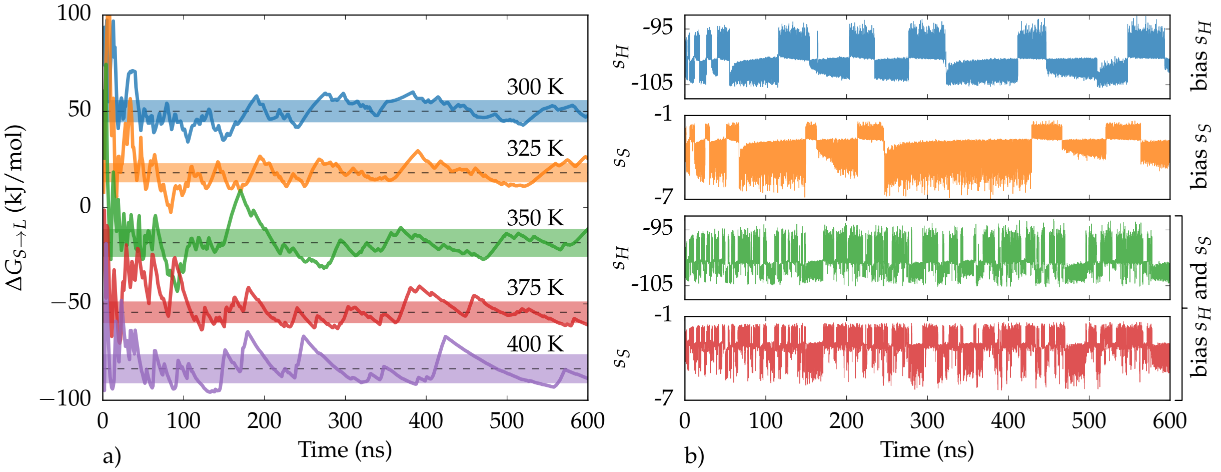


Figure SI-2: a) $\Delta G_{S\to L}$ as a function of simulation time for Na. For each temperature, the mean value and the deviation of $\Delta G_{S\to L}$ in the interval [100:600] are also depicted. b) CVs as a function of simulation time. The two uppermost plots corresponds to simulations in which only $s_H$ or $s_S$ were biased. The two lowermost plots correspond to a simulation in which both $s_H$ and $s_S$ were biased. It is clear that the sampling efficiency in the latter simulation is much greater. $s_H$ is expressed in kJ/mol and $s_S$ is in $k_B$.

as a function of temperature in Fig. 2 of the manuscript. The trajectories in $s_H$ and $s_S$ of the 350 K simulation are shown in Figure SI-2 b).

To demonstrate the usefulness of biasing together $s_S$ and $s_H$, we also performed simulations biasing only $s_S$ or $s_H$ (see Table 1). We show in Figure SI-2 b) that the individual efficiency of the CVs in metadynamics is very low. Instead if they are biased together the sampling efficiency is greatly improved.

**Variationally enhanced sampling**

We now turn to discuss the simulations performed with VES. Table 2 summarizes the simulations that were performed and the parameters that were employed. We calculated the FES from the VES simulations using,

$$V(s_H, s_S) = -F(s_H, s_S) - \frac{1}{\beta} \log p(s_H, s_S). \tag{8}$$

where $p(s_H, s_S)$ is the so called target distribution[6]. Convergence of the simulation was assessed in several ways. I) The evolution of the coefficients in the expansion of $V(s_H, s_S)$ was plotted as a function of time. At convergence the average coefficients become stationary as can be seen in Figure SI-3 a) for the 5 largest coefficients (absolute

Table 2: Simulations of Na performed with variationally enhanced sampling. Summary of the parameters that were used: target temperature of the thermostat ($T$), bias factor of the well tempered target distribution[7] ($\gamma$), step size in the optimization[6] ($\mu$), stride in the optimization[6] (stride), number of basis functions in $s_H$ (# $f_{s_H}$) and $s_S$ (# $f_{s_S}$), intervals in which the basis functions are defined in $s_H$ ($I_{s_H}$) and $s_S$ ($I_{s_S}$), number of walkers, and total simulation time per replica ($t$). In the first entry of the table we show all different temperatures for which the same parameters have been used.

| T (K) | $\gamma$ | $\mu$ (kJ/mol) | stride | # $f_{s_H}$ | # $f_{s_S}$ | $I_{s_H}$ (kJ/mol) | $I_{s_S}$ ($k_B$) | # walkers | $t$ (ns) |
|---|---|---|---|---|---|---|---|---|---|
| 300, 325, 350, 375, 400 | 50 | 5 | 500 | 40 | 40 | [-108,-92] | [-6.5,-1] | 6 | 450 |

values) in the simulation at 350 K. II) The FES was observed at different simulation times. When the simulation is converged the FES does not change substantially anymore. III) We also calculated $\Delta G_{S\to L}$ as a function of simulation time per replica. Figure SI-3 b) shows that after around 200 ns $\Delta G_{S\to L}$ fluctuates around a mean value. IV) When considering convergence, the observation of multiple recrossings between different basins, is crucial for the determination of a converged free energy surface. For this reason, in Fig. SI-3 c) and d) we show the trajectories of the 6 multiple walkers employed in the 350 K simulation. It is observed that all the multiple walkers make multiple transitions between the liquid and bcc phases.

## 2.2 Determination of melting temperature and entropy of fusion

Once that $\Delta G_{S\to L}$ is known as a function of temperature, the melting temperature $T_m$ can be calculated from $\Delta G_{S\to L}(T_m) = 0$. In Fig. 2 of the manuscript, we show the result of fitting a straight line to the WTMetaD data points. We only employed the data points at temperatures 325, 350 and 375 K due to their proximity to the melting temperature. From this line, we estimate $T_m$ to be around 340 K. A similar estimation can be extracted from the VES simulations.

The entropy of fusion $\Delta S_{S\to L}$ was calculated using two different procedures.

- We computed the slope of the straight line fitted to calculate the melting temperature and used the thermodynamic relation:

$$\Delta S_{S\to L} = -\frac{\partial \Delta G_{S\to L}}{\partial T}\Big|_{N,P}. \tag{9}$$

  We obtained $\Delta S_{S\to L} = 5.8$ J K$^{-1}$ mol$^{-1}$.

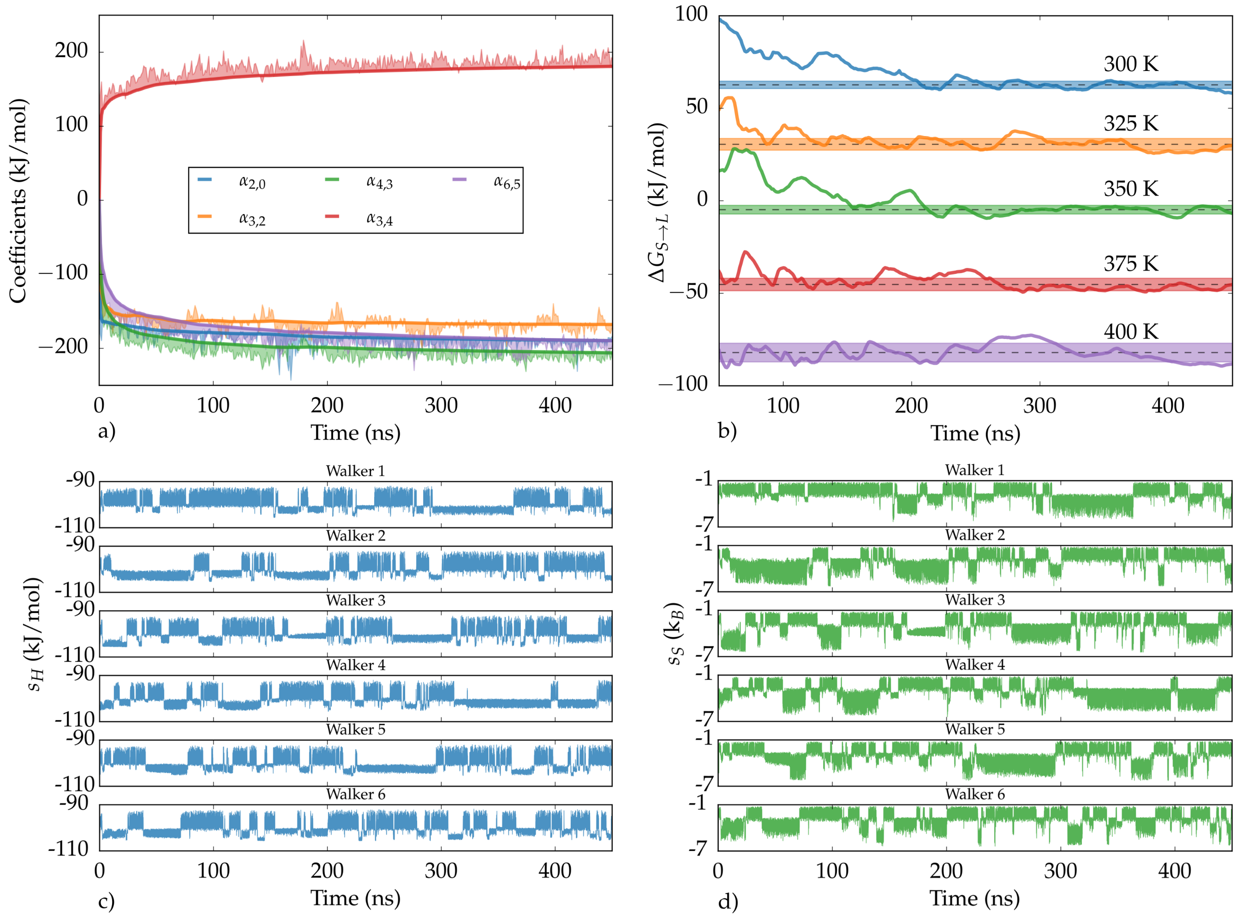


Figure SI-3: Simulations of Na using VES. a) Evolution of selected coefficients with simulation time (per replica). b) Convergence of $\Delta G_{S\to L}$ with simulation time for different temperatures. c) and d) Trajectories of multiple walkers in $s_H$ (kJ/mol) and $s_S$ ($k_B$).

- We calculated the enthalpy per atom of the liquid and solid at 350 K (close to the melting temperature) using the position of the minima of the FES. We obtained $\Delta H_{S\to L} = 2.24$ kJ/mol. We then employed the definition of Gibbs free energy $\Delta G_{S\to L} = \Delta H_{S\to L} - T\Delta S_{S\to L}$ to calculate $\Delta S_{S\to L}$ as:

$$\Delta S_{S\to L} = \frac{\Delta H_{S\to L} - \Delta G_{S\to L}}{T} \tag{10}$$

  and employed $\Delta G_{S\to L} = -0.073$ kJ/mol calculated using equation (7). We obtained $\Delta S_{S\to L} = 6.6$ J K$^{-1}$ mol$^{-1}$.

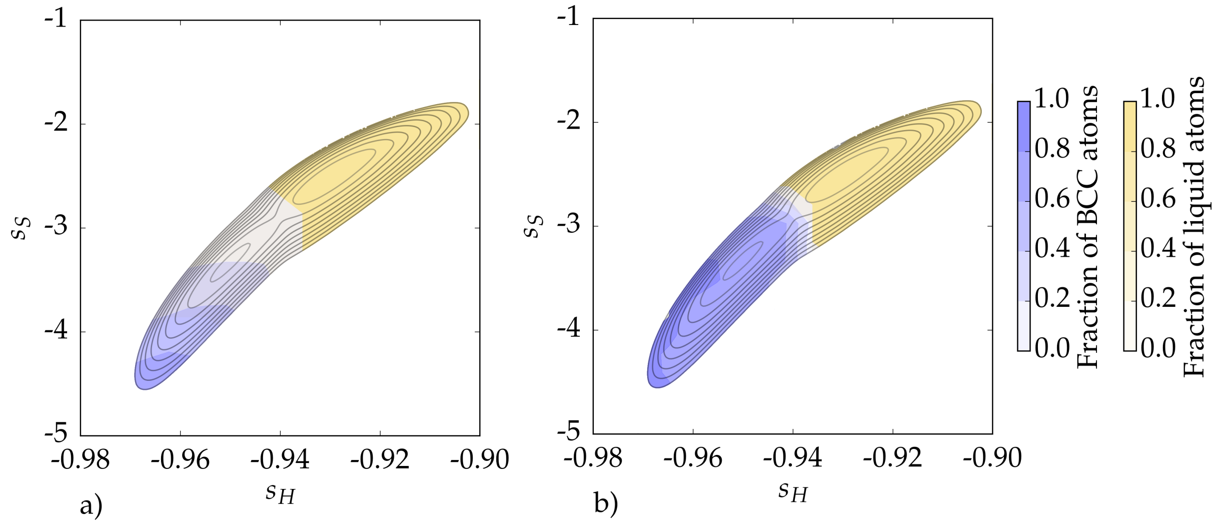


Figure SI-4: Average fraction of liquid and bcc-like atoms as a function of $s_H$ and $s_S$ calculated with CNA. The free energy surface is shown with contour lines. Subfigure a) corresponds to the calculation using the WTMetaD trajectory as obtained from the simulation whereas results in subfigure b) were obtained after the energy of each configuration in the trajectory was minimized with respect to the atomic coordinates.

## 2.3 Analysis of the solid structures

The different phases that appear in the WTMetaD simulation at 350 K were studied using the adaptive version of common neighbor analysis (CNA)[8,9]. The average fractions of bcc-like ($\langle \text{bcc} \rangle$) and liquid-like ($\langle \text{liq} \rangle$) atoms are shown in Fig. SI-4 as a function of the CVs. The results in Fig. SI-4 a) correspond to the calculation using the trajectory as obtained from the simulation whereas the results in Fig. SI-4 b) were obtained after the energy of each configuration in the trajectory was minimized with respect to the atomic coordinates. We have also plotted contour lines of the FES superimposed to the fraction of the different phases. Two basins are clearly seen from the contour plots. Each basin has a well defined character, either bcc or liquid. Only a negligible fraction of other solid phases were found in the trajectories. In SI-4 a) is is seen that $\langle \text{bcc} \rangle$ shows a strong correlation with $s_S$ . The minimum of the bcc basin in this figure has a relatively low $\langle \text{bcc} \rangle (\sim 0.3)$ as a result of thermal noise, and the formation of structures with one or a few vacancies. On the other hand, the quenched bcc configurations analyzed in SI-4 b) have a high $\langle \text{bcc} \rangle$ ($\sim 0.8$) in most of the basin. We note that the ability of the CVs to distinguish between the two phases is clearly seen from this figure.

Table 3: Simulations of Al performed with well tempered metadynamics. Summary of the parameters that were used: target temperature of the thermostat ($T$), biased CVs (CVs), bias factor of the well tempered distribution ($\gamma$), height of the gaussians ($w$), deviation of the gaussians in $s_H$ ($\sigma_{s_H}$), deviation of the gaussians in $s_S$ ($\sigma_{s_S}$), number of walkers, and total simulation time ($t$). In the first entry of the table we show all different temperatures for which the same parameters have been used.

| $T$ (K) | CVs | $\gamma$ | $w$ (kJ/mol) | $\sigma_{s_H}$ (kJ/mol) | $\sigma_{s_S}$ ($k_B$) | # walkers | $t$ (ns) |
|---|---|---|---|---|---|---|---|
| 700, 750, 800, 850 | $s_H, s_S$ | 30 | 7.5 | 0.3 | 0.1 | 1 | 800 |
| 900 | $s_H, s_S$ | 30 | 7.5 | 0.2 | 0.1 | 1 | 800 |

# 3 Aluminum

We simulated Al using the embedded atom model (EAM) reported in ref. 10. Two EAM potentials for Al were developed in that article and we have employed the one they name Al1. This model has a melting temperature of 926 K according to their calculation and fcc is the minimum potential energy structure. The cohesive energy of the fcc lattice is $E_{\mathrm{coh}}$ = 3.411 eV/atom = 329.11 kJ/mol/atom.

## 3.1 Calculation of the Gibbs free energy surface

We calculated the FES $F(s_H, s_S)$ for Al at different temperatures using WTMetaD. Details of the simulations that were carried out are shown in Table 3.

In Figure SI-5 we show $P(s_H, s_S)$ for the all studied temperatures. The procedure for the calculation of $P(s_H, s_S)$ was the same as the one used for Na. Figure SI-5 shows only one region of high probability at 700 K corresponding to the solid state. Between 750 K and 850 K there are two regions of high probability associated to the solid and the liquid states. At 900 K only the liquid state region is present. From this plots the melting temperature can be estimated to be around 800 K since at this temperature the two states have a similar probability. The structures in the solid basin are predominantly fcc, albeit a few structures with stacking faults do form in the trajectories.

As for Na, $\Delta G_{S\to L}$ was calculated for Al as a function of simulation time using equation (7). The results for the five studied temperatures are shown in Figure SI-6 a). The mean value and deviation of $\Delta G_{S\to L}$ are plotted as a function of temperature in Fig. 2 of the manuscript. Figure SI-6 b) shows the trajectory in CV space of the 800 K simulation. The exploration of the CV space is thorough and the system transforms many times reversibly between the different states.

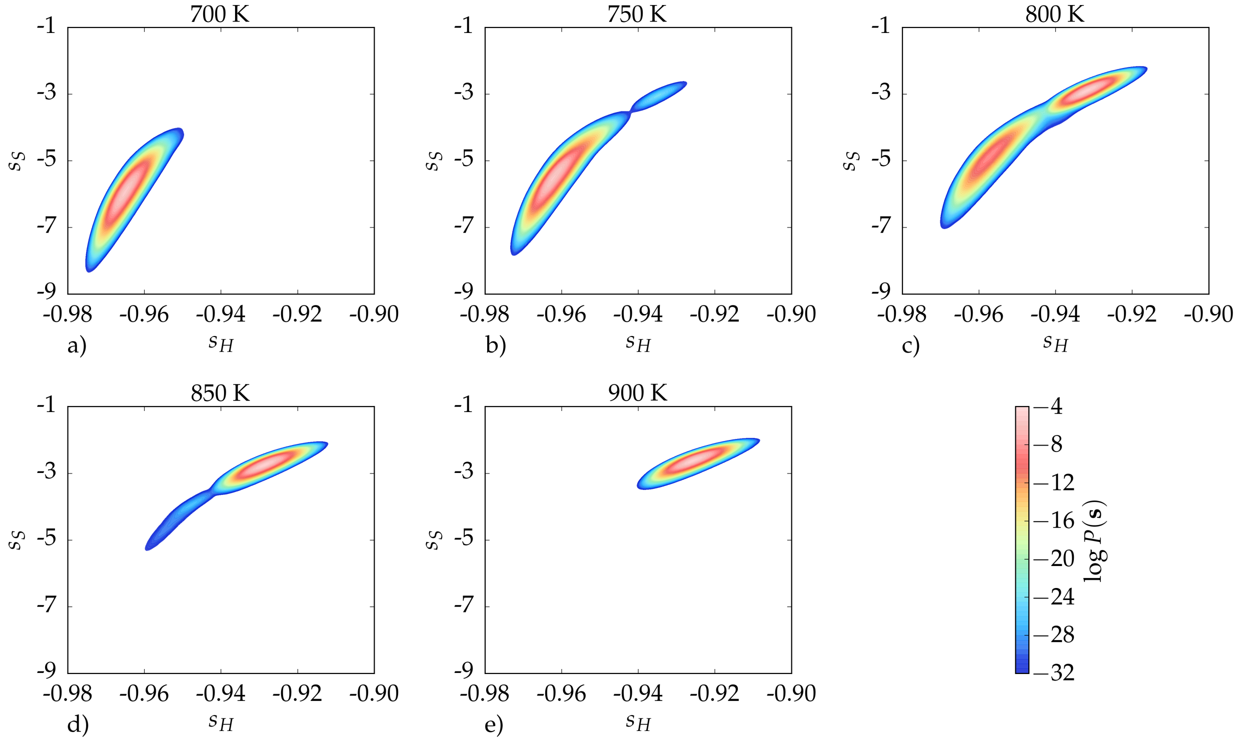


Figure SI-5: a)-e) Marginal probability distribution with respect to $s_H$ and $s_S$ for temperatures in the range 700-800 K for Al. $s_H$ is expressed in units of the cohesive energy and $s_S$ is in $k_B$.

## 3.2 Determination of melting temperature and entropy of fusion

The melting temperature $T_m$ of Al was calculated from the condition $\Delta G_{S\to L}(T_m) = 0$, as done for Na. In Fig. 2 of the manuscript, we show the result of fitting a straight line to the WTMetaD data points. We only employed the data points at temperatures 750, 800 and 850 K due to their proximity to the melting temperature. From this line, we estimate $T_m$ to be around 800 K.

As before, the entropy of fusion $\Delta S_{S\to L}$ was calculated using two different procedures.

- We computed the slope of the straight line fitted to calculate the melting temperature and used equation (9) to obtain $\Delta S_{S\to L} = 9.5$ J K$^{-1}$ mol$^{-1}$.
- We calculated the enthalpy per atom of the liquid and solid at 800 K using the position of the minima of the FES. We obtained $\Delta H_{S\to L} = 8.595$ kJ/mol. We then employed equation (10) and $\Delta G_{S\to L} = -0.0021$ kJ/mol calculated using equation (7). We obtained $\Delta S_{S\to L} = 10.7$ J K$^{-1}$ mol$^{-1}$.

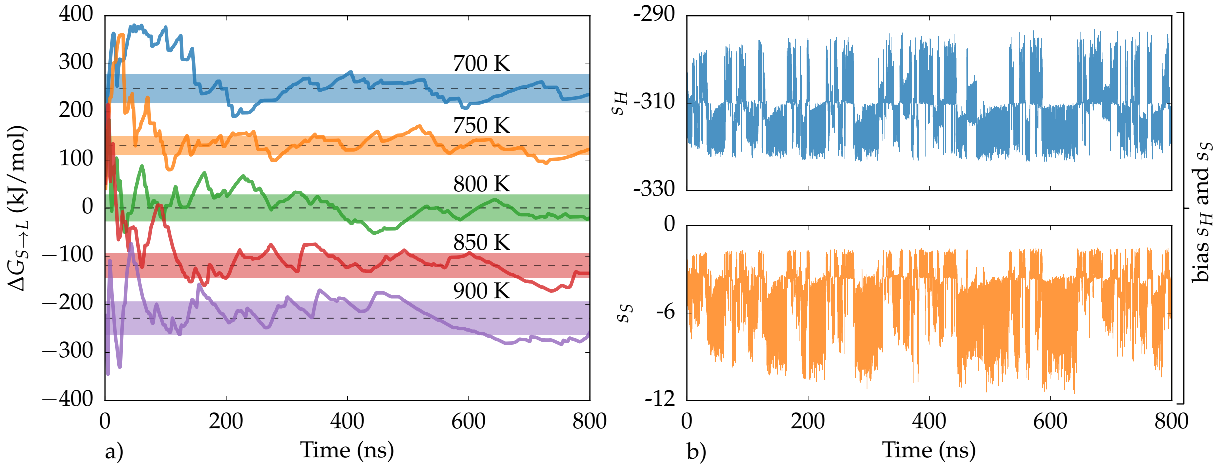


Figure SI-6: a) $\Delta G_{S\to L}$ as a function of simulation time for Al. For each temperature, the mean value and the deviation of $\Delta G_{S\to L}$ in the interval [100:800] are also depicted. b) CVs as a function of simulation time. The two plots correspond to a simulation in which both $s_H$ and $s_S$ were biased. $s_H$ is expressed in kJ/mol and $s_S$ is in $k_B$.

## 3.3 Analysis of the solid structures

We studied the solid structures in the WTMetaD trajectory at 800 K using CNA. Figure SI-7 shows the average fraction of fcc-like ($\langle$fcc$\rangle$), bcc-like ($\langle$bcc$\rangle$), and liquid-like ($\langle$liq$\rangle$) atoms as a function of $s_H$ and $s_S$. We also plotted contour lines of the FES superimposed to the fraction of the different phases. Two basins and a broad shoulder are seen in the contour plot. The solid basin has a high $\langle$fcc$\rangle$ and at the FES minimum $\langle$fcc$\rangle \sim 0.5$. Some atoms do not have fcc character due to thermal noise, formation of vacancies, and voids (see below) The average fraction of hcp-like atoms ($\langle$hcp$\rangle$) is not shown but is very low compared to $\langle$fcc$\rangle$ ($\langle$hcp$\rangle < 0.15\,\forall\, s_H, s_S$). The shoulder in the contour plot has a strong bcc character. The bcc phase can therefore be found at very high free energies, but since there is no minimum, it is unstable. Configurations with bcc structure loose the bcc character after minimizing the potential energy with respect to the atomic coordinates. We therefore do not show the average fraction of each structure after the minimization as done for Na. We note that to distinguish between liquid, fcc, and bcc both $s_H$ and $s_S$ are necessary.

Some of the fcc configurations formed during the simulations have relatively large voids such as the one shown in Figure SI-8 a). Figure SI-8 b) shows a slice of the configuration in Figure SI-8 a). The nature of the voids can be seen in this Figure. To test the stability of these voids, a configuration with a void was simulated using an anisotropic barostat for 1 ns. The void remains throughout the simulation proving that these structures can form and that they have a relatively long lifetime. Structures

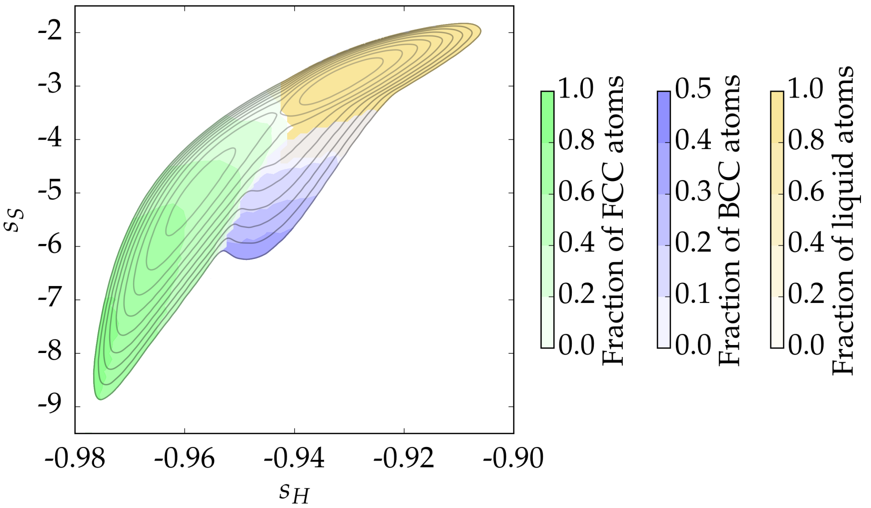


Figure SI-7: Average fraction of liquid, fcc-like, and bcc-like atoms as a function of $s_H$ and $s_S$ calculated with CNA. The free energy surface is shown with contour lines.

with voids are also local minima of the potential energy surface since voids also subsist after energy minimization. This indicates a possible pitfall of this potential. Finding this artifact was only made possible by the use of an enhanced sampling method.

# References

[1] M. Bonomi and M. Parrinello, *Physical review letters*, 2010, **104**, 190601.

[2] G. A. Tribello, M. Bonomi, D. Branduardi, C. Camilloni and G. Bussi, *Computer Physics Communications*, 2014, **185**, 604–613.

[3] S. Wilson, K. Gunawardana and M. Mendelev, *The Journal of chemical physics*, 2015, **142**, 134705.

[4] A. Laio and M. Parrinello, *Proceedings of the National Academy of Sciences*, 2002, **99**, 12562–12566.

[5] A. Barducci, G. Bussi and M. Parrinello, *Physical review letters*, 2008, **100**, 020603.

[6] O. Valsson and M. Parrinello, *Physical review letters*, 2014, **113**, 090601.

[7] O. Valsson and M. Parrinello, *Journal of chemical theory and computation*, 2015, **11**, 1996–2002.

[8] A. Stukowski, *Modelling and Simulation in Materials Science and Engineering*, 2009, **18**, 015012.

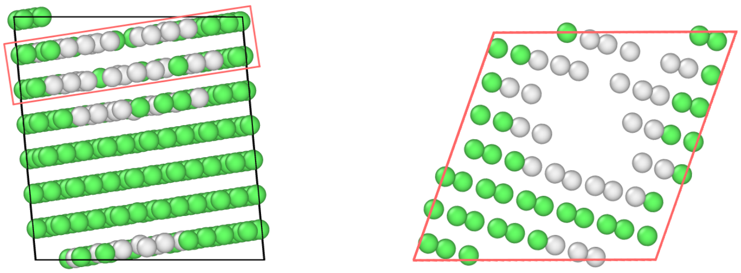

a) b)

Figure SI-8: Void in the fcc phase of the Al model studied in this work. a) Configuration with void. b) Slice of the configuration in a) in which the void is clearly observed. The structures were identified using CNA. Fcc-like atoms are colored in green and atoms without a known structure are colored in white.


[9] J. D. Honeycutt and H. C. Andersen, *Journal of Physical Chemistry*, 1987, **91**, 4950–4963.

[10] M. Mendelev, M. Kramer, C. A. Becker and M. Asta, *Philosophical Magazine*, 2008, **88**, 1723–1750.
